# Supplementary material for: Query Generation Pipeline with Enhanced Answerability Assessment for Financial Information Retrieval
Source: arXiv:2511.05000 source file (2025-11-07)
Supplement: Supplementary file 1 [file 6_Appendix.tex]

\section{Example of Bank product Document}
\label{sec:Examplebankproduct}
In this section, we present an example document sample in Figure~\ref{fig:sample_document}. Additionally, Table~\ref{tab:product_name_list} lists the 48 Kakaobank financial products used as data sources. Figure~\ref{fig:hierarchical_structure} illustrates the hierarchical structure of the financial document dataset constructed for the KoBankIR benchmark. Since financial documents often contain overlapping content across products, each document is treated independently. Metadata—product name, document title, and last modified date—is added to each passage to ensure disambiguation.

\begin{figure*}[h!]
\centering
  \includegraphics[width=0.85\linewidth]{Figures/sample_document.pdf}
  \caption{An example screenshot of the KakaoBank Time Deposit product description.}
  \label{fig:sample_document}
\end{figure*}

\newpage
\onecolumn
\begin{table}[h!]
\centering
\footnotesize

\begin{tabular}{|r|l|l|}
\hline
\multicolumn{1}{|l|}{} & \textbf{Product Name (Korean)}  & \textbf{Product Name (English)}                                   \\ \hline
1                      & \textbf{카카오뱅크\_정기예금}             & KakaoBank Fixed Deposit                                           \\ \hline
2                      & \textbf{카카오뱅크\_미니(mini)}         & KakaoBank Mini                                                    \\ \hline
3                      & \textbf{카카오뱅크\_자유적금}             & KakaoBank Free Savings                                            \\ \hline
4                      & \textbf{카카오뱅크\_특별판매\_정기예금}        & KakaoBank Special Time Deposit                                   \\ \hline
5                      & \textbf{mini\_생활\_서비스}            & Mini Lifestyle Services                                           \\ \hline
6                      & \textbf{카카오뱅크\_개인사업자\_보증서대출(비대면)} & KakaoBank SME Guarantee Loan (Non-face-to-face)                   \\ \hline
7                      & \textbf{대출비교\_서비스}               & Loan Comparison Service                                           \\ \hline
8                      & \textbf{주택담보대출\_갈아타기}            & Mortgage Refinancing Loan                                         \\ \hline
9                      & \textbf{카카오뱅크\_내\_사업장\_신용정보}       & KakaoBank My Business Credit Information                          \\ \hline
10                     & \textbf{카카오뱅크\_주택담보대출}           & KakaoBank Mortgage Loan                                           \\ \hline
11                     & \textbf{카카오뱅크\_마이너스\_통장대출}        & KakaoBank Overdraft Loan                                          \\ \hline
12                     & \textbf{카카오뱅크\_내\_신용정보\_서비스}       & KakaoBank My Credit Information Service                           \\ \hline
13                     & \textbf{카카오뱅크\_개인사업자\_체크카드}       & KakaoBank SME Check Card                                          \\ \hline
14                     & \textbf{카카오뱅크\_저금통}              & KakaoBank Savings Jar                                             \\ \hline
15                     & \textbf{카카오뱅크\_중신용플러스대출}         & KakaoBank Mid-Credit Plus Loan                                    \\ \hline
16                     & \textbf{카카오뱅크\_중신용비상금대출}         & KakaoBank Mid-Credit Emergency Loan                               \\ \hline
17                     & \textbf{국세청\_사업용\_계좌(카드)\_등록\_서비스}  & National Tax Service Business Account (Card) Registration Service \\ \hline
18                     & \textbf{신용대출\_갈아타기}              & Credit Loan Refinancing                                           \\ \hline
19                     & \textbf{카카오뱅크\_개인사업자\_보증서대출(대면)}  & KakaoBank SME Guarantee Loan (Face-to-face)                       \\ \hline
20                     & \textbf{카카오뱅크\_전월세보증금\_대출}        & KakaoBank Jeonse Deposit Loan                                     \\ \hline
21                     & \textbf{카카오뱅크\_비상금대출}            & KakaoBank Emergency Loan                                          \\ \hline
22                     & \textbf{카카오뱅크\_중신용대출}            & KakaoBank Mid-Credit Loan                                         \\ \hline
23                     & \textbf{전월세보증금\_대출\_갈아타기}         & Jeonse Deposit Loan Refinancing                                   \\ \hline
24                     & \textbf{카카오뱅크\_서베이\_서비스}          & KakaoBank Survey Service                                          \\ \hline
25                     & \textbf{금융정보\_구독\_서비스}            & Financial Information Subscription Service                        \\ \hline
26                     & \textbf{카카오뱅크\_26주적금}            & KakaoBank 26-Week Installment Savings                                         \\ \hline
27                     & \textbf{카카오뱅크\_신용대출}             & KakaoBank Credit Loan                                             \\ \hline
28                     & \textbf{카카오뱅크\_한달적금}             & KakaoBank One-Month Savings                                       \\ \hline
29                     & \textbf{카카오뱅크\_개인사업자통장}          & KakaoBank SME Account                                             \\ \hline
30                     & \textbf{카카오뱅크\_프렌즈\_체크카드}         & KakaoBank Friends Check Card                                      \\ \hline
31                     & \textbf{카카오뱅크\_세이프박스}            & KakaoBank Safe Box                                                \\ \hline
32                     & \textbf{카카오뱅크\_증권계좌개설서비스}        & KakaoBank Securities Account Opening Service                      \\ \hline
33                     & \textbf{증권계좌개설서비스(NH투자증권)}      & Securities Account Opening Service (NH Investment \& Securities)   \\ \hline
34                     & \textbf{카카오뱅크\_기록통장}             & KakaoBank Record Account                                          \\ \hline
35                     & \textbf{카카오뱅크\_달러박스\_서비스}         & KakaoBank Dollar Box Service                                      \\ \hline
36                     & \textbf{카카오뱅크\_모임\_체크카드}          & KakaoBank Group Check Card                                        \\ \hline
37                     & \textbf{카카오뱅크\_오픈뱅킹}             & KakaoBank Open Banking                                            \\ \hline
`38                     & \textbf{카카오뱅크\_모임통장}             & KakaoBank Group Account                                           \\ \hline
39                     & \textbf{카카오뱅크\_개인사업자\_대출}         & KakaoBank SME Loan                                                \\ \hline
40                     & \textbf{전자금융서비스\_이용약관}           & Electronic Financial Service Terms of Use                         \\ \hline
41                     & \textbf{카카오뱅크\_해외송금}             & KakaoBank Overseas Remittance                                     \\ \hline
42                     & \textbf{중고차\_구매대출}               & Used Car Purchase Loan                                            \\ \hline
43                     & \textbf{똑똑한\_구독생활}               & Smart Subscription Life                                           \\ \hline
44                     & \textbf{브랜드쿠폰서비스}               & Brand Coupon Service                                              \\ \hline
45                     & \textbf{카카오뱅크\_부가세박스}            & KakaoBank VAT Box                                                 \\ \hline
46                     & \textbf{카카오뱅크\_입출금통장}            & KakaoBank Transaction Account                                     \\ \hline
47                     & \textbf{카카오뱅크\_앱카드}              & KakaoBank App Card                                                \\ \hline
48                     & \textbf{카카오뱅크\_mini카드}           & KakaoBank Mini Card                                               \\ \hline
\end{tabular}
\caption{List of Kakaobank's product names}
\label{tab:product_name_list}
\end{table}
\twocolumn

\begin{figure}[h!]
\centering
  \includegraphics[width=0.85\linewidth]{Figures/financial document category.pdf}
  \caption{Hierarchical Structure of the Financial Document Dataset.}
  \label{fig:hierarchical_structure}
\end{figure}

\section{Experimental Details}

To investigate performance differences across the three types of retrieval models using our benchmark, we designed a comprehensive experimental setup. All the experiments were conducted using a single NVIDIA RTX3090 GPU. The results are shown in Table~\ref{table:Experimental results}. We use the okapi BM25 algorithm using rank\_bm25\footnote{\url{https://github.com/dorianbrown/rank_bm25}} python package. For pre-trained models, we directly use their checkpoints in huggingface\footnote{\url{https://huggingface.co/}}. The numbers of parameters of the models we used are listed in Table~\ref{tab:model_params}. 

\begin{table}[h]
\centering
\footnotesize
\begin{tabular}{l|r}
\toprule
Model                                   & \# of Parameters \\ \hline
Alibaba-NLP/gte-Qwen2-1.5B-instruct     & 568M            \\ \hline
intfloat/multilingual-e5-large          & 560M            \\ \hline
intfloat/multilingual-e5-large-instruct & 560M            \\ \hline
BAAI/bge-m3                    & 1.5B           \\ \bottomrule
\end{tabular}
\caption{The number of parameters of the models used in our experiments.}
\label{tab:model_params}
\end{table}

\section{KoBankIR Dataset}
\label{sec:kobankir_dataset}
The KoBankIR dataset consists of 815 queries curated for the benchmark, comprising 457 single-document queries and 358 multi-document queries. The multi-document queries are further categorized into three types: Topic-based Merging, Context Deepening, and Comparing and Contrasting (see Table~\ref{tab:data_stat2}). Figure~\ref{fig:Token_lengths} illustrates the token length distributions of both the queries and their associated documents, providing insights into the linguistic complexity and contextual diversity present in the dataset.

% \clearpage
\section{ThinkEval}
\label{sec:ThinkEval process}

Figure~\ref{fig:ThinkEval process} presents the pipeline of the ThinkEval evaluation framework, which guides LLMs to perform explicit reasoning to assess the answerability of questions based on structured prompt instructions. When ThinkEval with vLLM is running on two RTX 3090 Ti GPUs, the evaluation takes approximately 30 seconds per query. 

To support the human evaluation of query answerability on KoBankIR dataset, we adopt a 3-point rating scale aligned with the QGEval framework. Annotators assign scores based on how well each question can be answered using only the information provided in the associated passage. Table~\ref{tab:answerability_criteria} describes the scoring criteria used in this process.

\begin{table}[h!]
\centering
\begin{center}
\scriptsize

\begin{tabular}{p{0.2\columnwidth} p{0.7\columnwidth}}
\toprule
\textbf{Answerability} & \textbf{Criteria} \\
\midrule
Score 1 & The question cannot be answered based on the provided passage.\\
\midrule
Score 2 & The question can be partially answered based on the provided passage, or the answer to the question can be inferred to some extent.\\
\midrule
Score 3 & The question can be answered definitively based on the given passage.\\
\midrule
\end{tabular}
\caption{Answerability Scoring Criteria for Query Evaluation}
\label{tab:answerability_criteria}
\end{center}
\end{table}

% \clearpage
\section{LLM Prompts}
\label{sec:Prompts}
In this section, we provide the prompts used for the GPT-4o (\textit{2024-08-01-preview}) model deployed on Azure, which were utilized for both single-document and multi-document query generation.

To generate single-document queries, we designed a structured prompt that reflects real-world banking inquiry scenarios. We incorporate customer profiles to ensure that the queries generated align with actual customer interactions typically observed in banking environments. Each input passage was referenced directly within the scenario to create contextually appropriate queries. To ensure high-quality and stable query generation in Korean, the prompt template was constructed entirely in Korean. The actual prompt used for this process is shown in Figure ~\ref{fig:prompt0}.

For multi-document queries, we considered three types: topic-based merging, context-deepening, and comparing and contrasting, as introduced in \ref{sec:section3_2}. Each type involved a two-step prompting process: one prompt for selecting relevant candidate queries, and another for generating the final multi-document query based on those candidates. All prompt templates were written in Korean, maintaining consistency and improving the linguistic quality of the outputs.

The prompts used for topic-based merging queries are shown in Figure ~\ref{fig:prompt1} and Figure ~\ref{fig:prompt2}. For context deepening queries, the prompt templates are illustrated in Figure ~\ref{fig:prompt3} and Figure ~\ref{fig:prompt4}. Finally, the prompts designed for comparing and contrasting queries are provided in Figure ~\ref{fig:prompt5} and Figure ~\ref{fig:prompt6}.

% \newpage
\section{Human Evaluation}
\label{sec:human_eval}
To ease efforts of human annotator, we build an annotation interface described in Figure~\ref{fig:human_eval_interface}

\begin{figure*}[h!]
\centering
\includegraphics[width=0.95\linewidth]{Figures/token_lengths.png}
\caption{Token length.}
\label{fig:Token_lengths}
\end{figure*}

\begin{figure*}[h!]
\centering
  \includegraphics[width=0.95\linewidth]{Figures/ThinkEval_pipe.png}
  \caption{The process of ThinkEval.}
  \label{fig:ThinkEval process}
\end{figure*}
% \twocolumn

\onecolumn
\begin{table}[h]
\small
\centering

\begin{tabular}{p{0.25\linewidth} | p{0.6\linewidth} | c}
\toprule
\textbf{Query} & \textbf{Document Context} & \textbf{Score} \\
\midrule
\textbf{(english)} \newline
How much do I need to deposit each week over the 26-week period? \newline
\textbf{(korean)} \newline
26주 동안 매주 얼마를 납입해야 하나요?

& \textbf{(english)} \newline
\textbf{Product Name}: KakaoBank\_26-Week Installment Savings \newline
\textbf{Document Name}: KakaoBank\_26-Week Installment Savings Product Information.pdf \newline
\textbf{Last Updated}: January 1, 2025 \newline
\textbf{Chunk}: 5/8 \newline
\textbf{Context}: A 26-week installment savings plan in which you deposit an amount that increases each week by the original enrollment amount to build up a lump sum. \newline
\textbf{(korean)} \newline
\textbf{상품명}: 카카오뱅크\_26주적금 \newline
\textbf{문서명}: 카카오뱅크\_26주적금\_상품설명서.pdf \newline
\textbf{최종변경일} : 2025.01.01 \newline
\textbf{Chunk} : 5/8 \newline
\textbf{내용}: 상품개요: 26 주동안 매주 가입금액만큼 증액된 금액을 납입하여 목돈을 모으는 적금 상품 
& 1.85 \\
\hline

\textbf{(english)} \newline
How do I set the PIN for the KakaoBank Friends Check Card? \newline
\textbf{(korean)} \newline
카카오뱅크 프렌즈 체크카드의 비밀번호는 어떻게 설정하나요?

& \textbf{(english)} \newline
\textbf{Product Name}: KakaoBank\_Friends\_Check Card \newline
\textbf{Document Name}: CheckCard\_IndividualMember\_Terms.pdf \newline
\textbf{Last Updated}: November 4, 2024 \newline
\textbf{Chunk}: 5/38 \newline
\textbf{Context}: Article 7 (Card PIN):
 Members must register their card PIN with KakaoBank according to the procedures prescribed by the bank. When using the card at any merchant that has a separate agreement with KakaoBank regarding PIN usage, each transaction requires the member to enter the registered PIN. KakaoBank will authorize a PIN-based transaction only if the entered PIN matches the registered PIN. Members must always ensure that their PIN is not disclosed to any third party.
\newline
\textbf{(korean)} \newline
\textbf{상품명}: 카카오뱅크\_프렌즈\_체크카드 \newline
\textbf{문서명}: 체크카드\_개인회원\_약관.pdf \newline
\textbf{최종변경일} : 2024.11.04 \newline
\textbf{Chunk} :5/38 \newline
\textbf{내용}: 제 7 조 (카드의 비밀번호)
① 회원은 카카오뱅크가 정하는 방법에 따라 카드 비밀번호를 신고하여야 하며, 카카오뱅크와 비밀번호를 사용하기로 별도의 약정을체결한 가맹점에서 카드를 이용하는 경우 매 거래 시마다 카카오뱅크에 신고한 비밀번호를 직접 입력하여야 합니다.② 카카오뱅크는 비밀번호를 이용하는 거래시 회원이 입력한 비밀번호와 회원이 신고한 비밀번호를 대조하여 일치함이 인정될 경우에한하여 거래를 허용합니다.③ 회원은 제 1 항의 비밀번호가 타인에게 유출되지 않도록 항상 주의하여야 합니다.
& 1.45 \\
\bottomrule
\end{tabular}
\caption{Examples of low ThinkEval scores with queries and document contexts.}
\label{tab:thinkeval_failure_bilingual}
\end{table}

\begin{figure*}[h!]
\centering
  \includegraphics[width=0.75\linewidth]{Figures/prompt0.pdf}
  \caption{The prompt designed for single-document query generation.}
  \label{fig:prompt0}
\end{figure*}

\begin{figure*}[h!]
\centering
  \includegraphics[width=0.9\linewidth]{Figures/prompt1.pdf}
  \caption{The prompt designed for evaluating candidates to use in Topic-based merging.}
  \label{fig:prompt1}
\end{figure*}

\begin{figure*}[h!]
\centering
  \includegraphics[width=0.9\linewidth]{Figures/prompt2.pdf}
  \caption{The prompt designed for Topic-based merging multi-document query generation ($T_{merge}$).}
  \label{fig:prompt2}
\end{figure*}

\begin{figure*}[h!]
\centering
  \includegraphics[width=0.9\linewidth]{Figures/prompt3.pdf}
  \caption{The prompt designed for evaluating candidates to use in Context Deepening.}
  \label{fig:prompt3}
\end{figure*}

\newpage
\begin{figure*}[h!]
\centering
  \includegraphics[width=0.8\linewidth]{Figures/prompt4.pdf}
  \caption{The prompt designed for Context Deepening multi-document query generation ($T_{deep}$).}
  \label{fig:prompt4}
\end{figure*}

\begin{figure*}[h!]
\centering
  \includegraphics[width=0.8\linewidth]{Figures/prompt5.pdf}
  \caption{The prompt designed for evaluating candidates to use in Comparing and Contrasting.}
  \label{fig:prompt5}
\end{figure*}

\newpage
\begin{figure*}[h!]
\centering
  \includegraphics[width=0.9\linewidth]{Figures/prompt6.pdf}
  \caption{The prompt designed for Comparing and Contrasting multi-document query generation ($T_{comp}$).}
  \label{fig:prompt6}
\end{figure*}

\begin{figure*}[h!]
\centering
  \includegraphics[width=0.95\linewidth]{Figures/Human evaluation interface.png}
  \caption{Human evaluation interface.}
  \label{fig:human_eval_interface}
\end{figure*}
